# Supplementary material for: Electrically driving nuclear spin qubits with microwave photonic bangap resonators
Source: arXiv:1701.06650 source file (2017-01-23)
Supplement: Supplementary file 1 [file Sigillito_EDNMR_Supplementary_Information.pdf]

# Electrically driving nuclear spin qubits with microwave photonic bangap resonators: supplementary information

A. J. Sigillito,[1,*] A. M. Tyryshkin,[1] T. Schenkel,[2] A. A. Houck,[1] and S. A. Lyon[1]

[1] *Department of Electrical Engineering, Princeton University, Princeton, New Jersey 08544, USA*
[2] *Accelerator and Fusion Research Division, Lawrence Berkeley National Laboratory, Berkeley, California 94720, USA*
(Dated: January 20, 2017)

## PHOTONIC BAND GAP RESONATOR SIMULATION AND DESIGN

### ABCD Matrix Simulations

The photonic bandgap (PBG) resonators are made up of a series of transmission lines having variable impedance. They can be designed using a transfer matrix (also known as ABCD matrix) technique as described by Pozar [1].

In the transfer matrix formalism, each segment of the PBG resonator's transmission line is represented by its own 2×2 ABCD matrix. The whole device's ABCD matrix is then constructed by taking the product of all of the individual ABCD matrices while maintaining their order. The ABCD matrix for a coplanar transmission line of length, L, and characteristic impedance, $Z_C$ is [1]

$$\begin{pmatrix} A & B \\ C & D \end{pmatrix} = \begin{pmatrix} \cosh(\Gamma L) & Z_C \sinh(\Gamma L) \\ \sinh(\Gamma L)/Z_C & \cosh(\Gamma L) \end{pmatrix} \tag{1}$$

where $\Gamma$ is given by

$$\Gamma = \alpha + ik \tag{2}$$

with $\alpha$ being the attenuation constant and $k$ being the microwave propagation constant.

The device measured in this work only consists of three different transmission line geometries, labeled here as $T_A$, $T_B$, and $T_C$. Lines $T_A$ and $T_B$ make up the Bragg mirrors and are 4.2 mm long. The designed characteristic impedance of $T_A$ is 92 Ω whereas $T_B$ is 34 Ω. Transmission line $T_C$ is the defect. It has a designed impedance of 50 Ω and a length of 6 mm. The overall geometry of the device follows the pattern $(T_A - T_B) \times 5 - T_C - (T_B - T_A) \times 5$. After computing the ABCD matrix for this device, we convert it into the more standard S-Parameter matrix using the conversion [1]:

$$\begin{pmatrix} S_{11} & S_{12} \\ S_{21} & S_{22} \end{pmatrix} = \begin{pmatrix} \frac{A+B/Z_C-CZ_0-D}{A+B/Z_C+CZ_C+D} & \frac{2(AD-BC)}{A+B/Z_C+CZ_C+D} \\ \frac{2}{A+B/Z_C+CZ_C+D} & \frac{-A+B/Z_C-CZ_0+D}{A+B/Z_C+CZ_C+D} \end{pmatrix} \tag{3}$$

Comparing the simulated PBG resonator to the measured one, we find reasonable agreement as shown in Fig. 1. The error in the simulation arises primarily from uncertainty in the position of the sample relative to the coplanar waveguide. The simulation assumes no gap between the sample and the waveguide, but even micron-scale gaps would serve to increase the resonance frequency of the device.

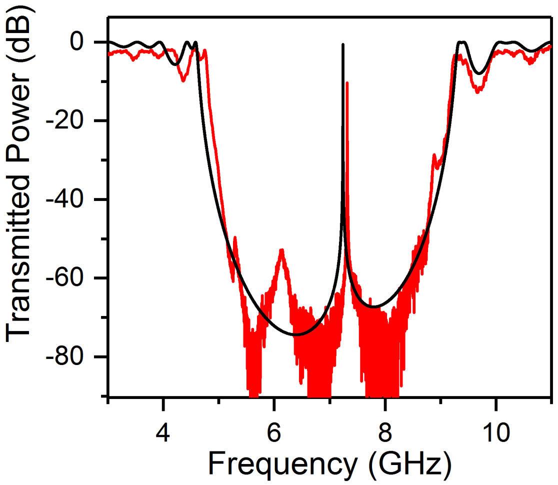


FIG. 1. Plot of transmitted microwave power through a device at 2 K in a magnetic field of 250 mT. The data (red) is compared to the simulated values (black).

### Design Considerations

There are several geometrical parameters that can be used to tune the resonator frequency, the resonator quality factor, the band gap depth, the band gap width and the band gap frequency. Qualitatively, these are outlined in Table I.

### Overcoming Inhomogeneous Fields

The electric and magnetic RF and microwave fields in the coplanar PBG resonator are inhomogeneous over the sample volume. The electric and magnetic field distributions in the photonic bandgap region can be calculated using conformal mapping techniques as described in [2]. We plot the typical fields expected in our device in Fig. 2.

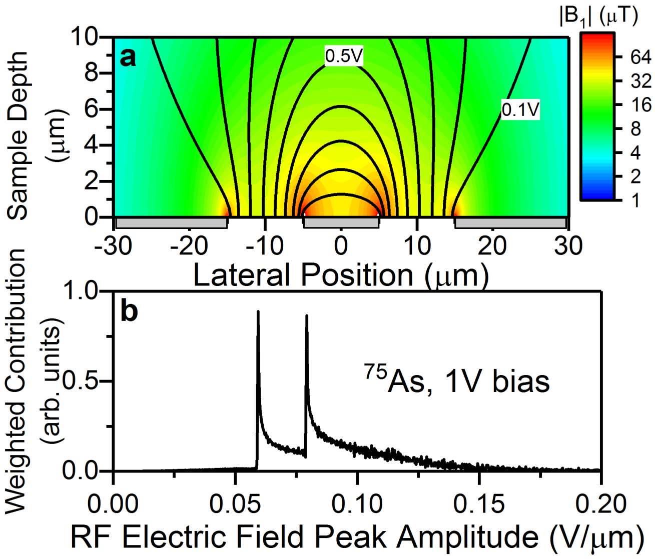


FIG. 2. (a) Density plot of the electric field at an antinode in $B_1$ assuming the signal has been optimized for 400 ns microwave $\pi$-rotations. The contours denote changes in the electric field potential (0.1 V/contour) assuming a 1 V bias on the center pin. The electric field distribution in the $^{75}$As spin ensemble (weighted by each spin's contribution to the echo) is plotted in (b). The two peaks correspond to sub-ensembles of spins located under the center pin and ground planes with the largest fields corresponding to spins under the center pin.

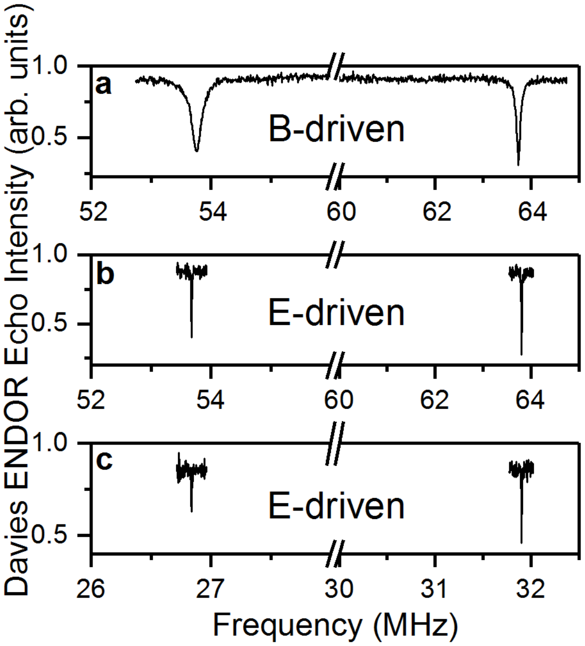


FIG. 4. Davies ENDOR spectra for the $^{31}$P donors. A conventional magnetically driven ENDOR spectrum is shown in (a) for the $M_I = +1/2$ hyperfine line. The EDNMR spectrum is shown in (b) and nuclear spins can be driven at subharmonics of these transitions as shown in (c). These data were taken at 1.9K in a field of 250 mT.

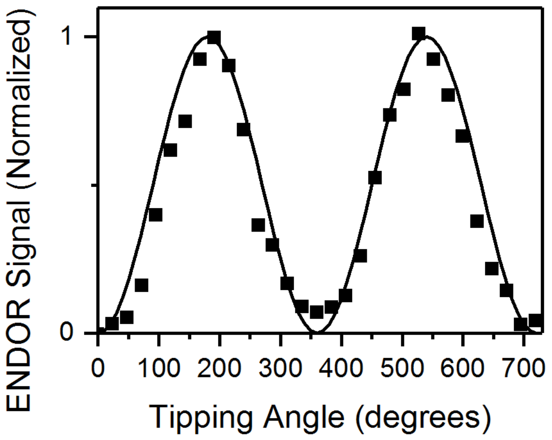


FIG. 3. The EDNMR signal is plotted as a function of the programmed tipping angle using the RF BIR-WURST pulse sequence. The data are represented by the square points whereas the ideal results are plotted as a solid line. Data is taken at 1.9 K in a field of 250 mT.

When measuring large ensembles of spins, microwave and RF inhomogeneities can complicate experiments by inducing spin tipping angle errors. These errors are partly responsible for the decay of Rabi oscillations in Fig. 4 of the main text. It has previously been shown that microwave magnetic field inhomogeneities can be easily overcome by incorporating adiabatic pulses as described in [3, 4]. Here we show that the similar pulse shapes can be used to overcome RF electric field inhomogeneity so that high-fidelity EDNMR can be performed in these structures. We use a WURST-20 (Wideband, Uniform Rate, Smooth Truncation 20 order) envelope shape with a BIR-4 ($B_1$ Insensitive Rotation 4th order) phase compensation. We find good results using a pulse envelope of 100 $\mu$s with a frequency chirp of 300 kHz as shown in Fig. 3. As can be seen in the figure, these pulses allow for very high fidelity EDNMR manipulations. This opens up the possibility of using PBG resonators to do complex EDNMR experiments requiring high fidelities at very low temperatures.

## DAVIES ENDOR OF $^{31}$P DONORS

Davies ENDOR experiments were performed on $^{31}$P donors in silicon using both magnetic and electrical RF fields. The spectra are plotted in Fig. 4. We only plot the ENDOR spectra for the $+1/2$ hyperfine line since the results were very similar for the $-1/2$ hyperfine line. As shown in the figure, EDNMR could be performed at both the fundamental and subharmonic frequencies of the transitions. The slight variation in transition frequencies for the three experiments comes from slight variations in the ESR resonator frequency, since the experiments were

conducted at slightly different magnetic fields. There is also a broadening observed for the lower frequency transition and the origin of this is currently unknown. This broadening also appears in the $-1/2$ hyperfine line. More experiments may be necessary to understand this lower frequency linewidth.

## DAVIES ENDOR RABI EXPERIMENT SIMULATION

The Rabi-type ENDOR experiment involves both RF and microwave pulses. The ENDOR signal is measured as a decrease in the electron spin echo signal while varying the amplitude and duration of the RF pulses that are resonant with nuclear spin transitions. Because there are distributions in the electric and magnetic fields, it was necessary to develop a model to simulate and understand the results of the Rabi frequency measurements described in the main text.

The ESR signal from a single spin at position $\vec{r}$ in a three pulse experiment $(\pi - T - \pi/2 - \tau - \pi - \tau - echo)$ is given by [5, 6]

$$signal(\vec{r}) = g_s(\vec{r}) sin^5(\tau_p g \beta B_1(\vec{r})/\hbar) \tag{4}$$

where $g_s(\boldsymbol{r})$ is the coupling of a spin at position $\vec{r}$ to the resonator, $\tau_p$ is the duration of the second pulse (nominally a $\pi/2$ pulse) in the sequence, $\beta$ is the Bohr magneton, $B_1$ is the magnitude of the microwave magnetic field orthogonal to $\vec{B}_0$, and $\hbar$ is the reduced Planck constant. $g_s$ can be calculated, but is proportional to $B_1(\vec{r})$ so in simulations we simply assume $g_s = B_1(\vec{r})$ and normalize the signal intensity.

Assuming ideal microwave pulses, the Davies ENDOR response from a single donor is simply given by $(1 - cos(\theta_E(\vec{r})))/2$ with $\theta_E(\vec{r})$ being the tipping angle of the nuclear spin due to the RF pulse. This tipping angle is given by the product of the nuclear Rabi frequency $(\omega_R)$ and the pulse length. The overall signal coming from the $i$th donor $(S_i)$ is therefore

$$S_i = AB_1(\vec{r}) sin^5(\tau_p g \beta B_1(\vec{r})/\hbar)(1 - cos(\theta_E(\vec{r}))) \tag{5}$$

where A is a normalization constant that also accounts for microwave losses in the detection channel. The overall ENDOR response of the donor spin ensemble $(S_{total})$ is then simply

$$S_{total} = \sum S_i \tag{6}$$

where the sum is taken over the doped region of the sample taking into account the doping profile shown in Fig. 2 of the main text. The only unknown parameter in the above model is the nuclear Rabi frequency. The Rabi frequency depends on the specific mechanism responsible for the electrically or magnetically driven NMR, so our model should be able to test which physical mechanism is responsible for the observed EDNMR transitions. We therefore turn our attention to the various mechanisms that can be responsible.

## ESTIMATION OF RABI FREQUENCIES FOR DIFFERENT PHYSICAL MECHANISMS

We identified three distinct effects that can lead to electrically driven nuclear magnetic resonance. The first arises from a modulation of the hyperfine interaction due to the hyperfine Stark effect, the second arises from the modulation of the electronic orbital states (which modulates the electron spin quantization axis), and finally, modulation of the nuclear quadrupole interaction.

As discussed in the main text, the subharmonic transitions should be more robust against strain compared to the fundamental transitions. We therefore focus the following discussion on the subharmonic transitions.

### Hyperfine Stark Effect Modulation

The hyperfine Stark shift is a modulation of the hyperfine tensor due to an applied electric field. Two effects must be considered — modulation of isotropic and anisotropic hyperfine components. Modulation of the isotropic hyperfine interaction follows the form $\Delta A/A = \eta_A E^2$ where $\eta_A$ is the hyperfine Stark shift parameter reported in Refs. [7–10]. The isotropic hyperfine interaction goes as $A\vec{S} \cdot \vec{I}$ and there is at least a two order of magnitude difference between the precession frequency of $\vec{S}$ and $\vec{I}$. In the rotating frame $S_X \cdot I_X = S_Y \cdot I_Y = 0$ and the only nonzero term is $A_{ZZ} S_Z \cdot I_Z$. This remaining term can not drive nuclear spin transitions.

$\overleftrightarrow{A}$ is isotropic for donors in silicon, even in the presence of strain and electric fields. Measurements of highly strained silicon [11] resolve no anisotropy in the hyperfine coupling so we do not expect modulation of an anisotropic hyperfine coupling to be responsible for the spin flips.

### Fluctuating Hyperfine Fields from $g$-Tensor Modulation of the Electronic Spin

One may be tempted to neglect modulation of the electronic spin-orbit interaction when considering electrically driven NMR since the spin-orbit interaction does not directly affect the nuclear spin. However, we show here that modulation of the electronic $g$-tensor in conjunction with an isotropic hyperfine interaction can lead to fluctuations in the hyperfine fields which lead to nuclear spin flips.

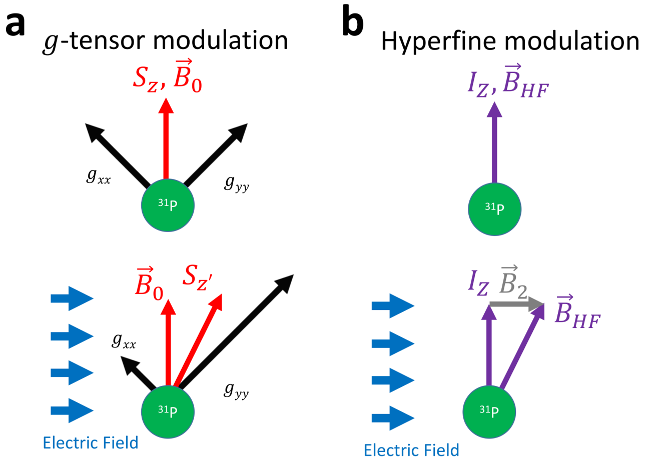


FIG. 5. Vector representation of the $g$-tensor modulation effect (a) which leads to a modulation of the hyperfine interaction (b). In the unperturbed case (top panels), the isotropic $g$-tensor ($g_{XX} = g_{YY} = g_{ZZ}$) results in the electronic spin quantizing along the direction of $\vec{B}_0$ (upwards). Likewise the nuclear spin is quantized along $\vec{B}_0$ and experiences an effective field due to the hyperfine interaction ($B_{HF}$) in that same direction. When an electric field is applied (lower panels) the $g$-tensor is made anisotropic ($g_{XX} \neq g_{YY}$) and the electronic spin is no longer quantized along $B_0$, but at some tilted angle. The hyperfine field seen by the nuclear spin is now also tilted resulting in a small effective $\vec{B}_2$ component orthogonal to $\vec{B}_0$ If the electric field modulation is done resonantly with the nuclear spin transition frequency, this can lead directly to spin flips.

In the absence of an externally applied electric field, the electronic $g$-tensor is isotropic and electron spins are quantized along the external magnetic field, $\vec{B}_0$ (Fig. 5(a), top). The nuclei are likewise quantized along $\vec{B}_0$ (Fig.5(b), top). When the electron spin is subjected to an AC electric field, the spin-orbit Stark effect modulates the $g$-tensor, thus tilting the quantization axis of the electron spin (Fig. 5(a), bottom) and by extension the hyperfine field of the electron (Fig. 5(c),bottom). It is important to note that the RF modulation frequency is much slower than the electron Zeeman frequency and the electron is in the slow passage regime. The electron spin and its hyperfine field follow the change in the quantization axis direction. As the electron spin tilts, the nuclear spin sees a hyperfine field ($\vec{B}_{HF}$) which changes its direction (Fig. 5(d), bottom) and has a component $\vec{B}_2$ perpendicular to the quantization axis of the nuclear spin. This component can excite nuclear spin transitions. Since the hyperfine interaction is large for donors in silicon, even small tilts in the electron spin can lead to a substantial $\vec{B}_2$ and rapid Rabi oscillations.

### *The Spin Hamiltonian*

A more quantitative analysis follows from the general spin Hamiltonian of Eq. 1 in the main text.

$$H = \beta B_Z \cdot \hat{g}(E,t) \cdot \vec{S} + \beta_n \cdot g_n \cdot B_Z \cdot I_Z + A_{iso} \cdot S_Z \cdot I_Z \quad (7)$$

After moving to a modulated $g$-tensor frame, where $g(E,t)$ is modulated by a resonant RF electric field, the Hamiltonian becomes

$$H = \nu_e S_{Z'} + \nu_n \cdot I_Z + A_{iso}(\cos(\delta(t)) \cdot S_{Z'} \cdot I_Z + \sin(\delta(t)) \cdot S_{Z'} \cdot I_X) \quad (8)$$

where $\nu_e$ and $\nu_n$ are the electronic and nuclear Zeeman frequencies, respectively, $Z'$ is the new electron quantization axis, and $\delta(t)$ is the time dependent tilting of the electron spin quantization axis. From this Hamiltonian, it is clear that if the $\delta(t)$ modulation is resonant with nuclear spin transitions, the $S_Z \cdot I_X$ term leads to nuclear Rabi oscillations. To determine the magnitude of $\delta$, we turn to the multi-valley effective mass theory of Wilson and Feher [12].

### *g-tensor modulation from valley repopulation*

Silicon has six conduction band valleys oriented along the (100) crystallographic axes. Each valley is ellipsoidal with an axially symmetric g tensor given by

$$\hat{g}_i = \begin{pmatrix} g_\perp & 0 & 0 \\ 0 & g_\perp & 0 \\ 0 & 0 & g_\parallel \end{pmatrix} \quad (9)$$

in the valley basis, with $g_\perp$ and $g_\parallel$ equal to the $g$ factors perpendicular and parallel to the valley axis, respectively. The overall g-tensor can be obtained by summing over each individual valley g-tensor weighted by the wavefunction amplitude in that valley so that in the molecular frame

$$\hat{g}_{eff} = \sum_{i=1}^{6} (\alpha_i)^2 R_{\vec{\theta}} \hat{g}_i \quad (10)$$

where $\hat{g}_{eff}$ is the overall $g$-tensor, $(\alpha_i)^2$ is the wavefunction amplitude in the $i$-th valley, and $R_{\vec{\theta}}$ is the set of rotation matrices that rotates $g_i$ to be in the crystal frame.

In the absence of an electric field, the $g$-tensor is isotropic and given by

$$g_{eff} = \begin{pmatrix} g_0 & 0 & 0 \\ 0 & g_0 & 0 \\ 0 & 0 & g_0 \end{pmatrix} \quad (11)$$

where $g_0$ is 1.99875 (1.99837) for $^{31}$P ($^{75}$As) donors in silicon[12]. The quantization axis $\vec{\Omega}$ of the electron spin is given by $\hat{g_{eff}} \cdot \vec{B}_0$ and for a $\langle 110 \rangle$ oriented magnetic field this becomes

$$\vec{\Omega} = \beta \cdot \begin{pmatrix} g_{xx} & 0 & 0 \\ 0 & g_{yy} & 0 \\ 0 & 0 & g_{zz} \end{pmatrix} \cdot \begin{pmatrix} B_0/\sqrt{2} \\ B_0/\sqrt{2} \\ 0 \end{pmatrix} \quad (12)$$

where $\beta$ is the Bohr magneton. Now, if we assume an electric field perturbation in the $\langle 001 \rangle$ direction, we can use the values for the valley populations derived by Wilson and Feher [12] which gives

$$(\alpha_A)^2 = 1/4[1 - (x + 2/3)(x^2 + 4/3x + 4)^{-1/2}] \quad (13)$$

$$(\alpha_B)^2 = 1/8[1 + (x + 2/3)(x^2 + 4/3x + 4)^{-1/2}] \quad (14)$$

where $(\alpha_A)^2$ and $(\alpha_B)^2$ are the wavefunction amplitudes for valleys along and orthogonal to the perturbing field, respectively and $x$ is the dimensionless "valley-strain" parameter which can be obtained by comparing Wilson and Feher's stress measurements with the electric field Stark shift measurements of [8] to find that $x = 0.203 \times E$ for $^{31}$P donors where E is in units of $V/\mu m$.

Given an electric field perturbation along $\langle 001 \rangle$, the $g$-tensor becomes

$$\hat{g}_{pert} = \begin{pmatrix} g_0 + \delta & 0 & 0 \\ 0 & g_0 + \delta & 0 \\ 0 & 0 & g_0 - 2\delta \end{pmatrix} \quad (15)$$

where $\delta = 2.5 \times 10^{-6}$ for a field of $0.1 V/\mu m$ and the precession axis of the electron spin becomes $\hat{g}_{pert} \cdot \vec{B}_0$. This corresponds to a quantization axis tilt of $1.9 \times 10^{-6}$ radians. Because the valley populations have a quadratic component, $\delta$ oscillates at twice the RF electric field frequency.

*Effect of $\delta$ on the hyperfine tensor*

A non-zero $\delta(t)$ leads to an $S_Z \cdot I_X$ term in the spin Hamiltonian as seen from Eq. 8. For completeness, we show here the full change to the hyperfine tensor given by a tilt in the quantization axis;

$$H_{HF} = \begin{pmatrix} S_x & S_y & S_z \end{pmatrix} \begin{pmatrix} \cos\delta(t) & 0 & -\sin\delta(t) \\ 0 & 1 & 0 \\ \sin\delta(t) & 0 & \cos\delta(t) \end{pmatrix} \begin{pmatrix} a_{iso} & 0 & 0 \\ 0 & a_{iso} & 0 \\ 0 & 0 & a_{iso} \end{pmatrix} \begin{pmatrix} I_x \\ I_y \\ I_z \end{pmatrix} \quad (16)$$

where the term that leads to EDNMR is the off-diagonal $A_{ZX}$ term. With the example field of 0.1 V/$\mu$m for $^{31}$P donors, the $A_{ZX}$ term becomes 330 Hz which is comparable to the values measured in experiment as illustrated in Fig. 4 of the main text.

When repeating this analysis for the $^{75}$As donors, theory predicts that the two donors should have comparable Rabi frequencies since $A_{iso}$ and $\eta_g$ are similar in both $^{75}$As and $^{31}$P . This contradicts our experimental observation of a 40× enhancement in the arsenic Rabi frequencies as shown in Fig.6. Given this discrepancy, we expect that a different mechanism is responsible for electrically driving the arsenic nuclei.

*Additional effects*

In addition to valley repopulation, there is a "single valley" Stark effect that is comparable in magnitude to the valley repopulation effect. The relative contributions of single-valley and valley repopulation effects to the $g$-tensor modulation varies depending on the direction of the RF fields in the sample, but given our geometry we expect the valley repopulation effect to be dominant. The spins probed in this experiment are subject to electric fields that are primarily oriented along a (100) equivalent direction. If the single valley effect was also taken into account, we would expect the Rabi frequencies to increase by as much as a factor of two, leading to better agreement between experiment and theory.

**Modulation of the Quadrupolar Interaction**

Phosphorus donors have $I = 1/2$ and do not have a nuclear quadrupole moment, so this mechanism only applies to the $^{75}$As donors ($I = 3/2$). There is nearly a two order of magnitude difference in the Rabi frequencies for $^{31}$P vs $^{75}$As donors and the quadrupole interaction in the only term in the spin Hamiltonian affecting $^{75}$As and not $^{31}$P. It is reasonable to expect that quadrupolar effects are enhancing the $^{75}$As nuclear spins' response to electric

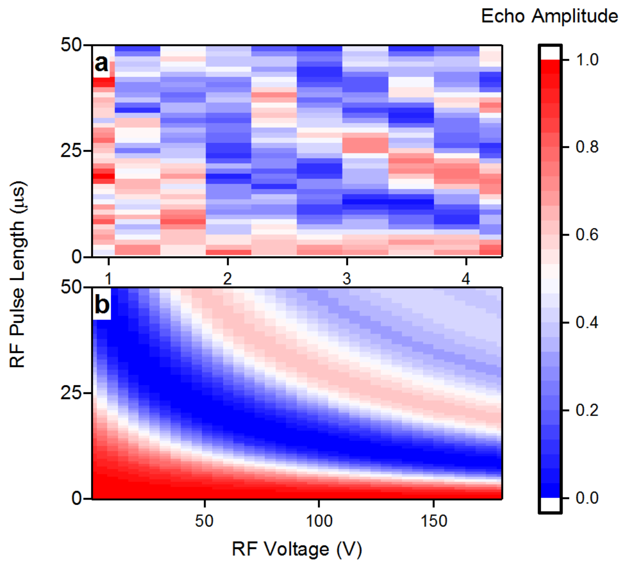


FIG. 6. Two dimensional plot of the Rabi oscillations for $^{75}$As donors(a) compared with theory(b). Note the difference in scale. Given the poor quality of fit, we are led to believe that another mechanism is responsible for the electrically driven NMR.

fields.

The quadrupolar coupling vanishes in the absence of strain or electric fields due to the cubic symmetry of the donor site. By applying RF electric fields, we are able to induce a field gradient at the nucleus which leads to a nonzero quadrupole coupling. More rigorous theory including knowledge of the electronic wavefunction at the nucleus will need to be developed to accurately determine how strongly electric fields can affect the quadrupole term, but we can make a crude approximation based on some recent experimental data. The experiments [13] measured the strain modulation of the quadrupole interaction on neutral $^{75}$As doped Si. The data report a quadrupolar shift of 65 kHz with a simultaneous hyperfine modulation of 1%. Based on the Stark effect measurements of [9], we can infer from the hyperfine shift an effective electric field due to strain of $\sim$3 V/$\mu$m. From this we can estimate the quadrupolar coupling induced in our experiments.

### *Driving transitions through modulation of $Q_{XX}$*

Quadrupolar coupling can lead to spin flips through direct modulation of the $Q_{XX}$ component of the quadrupolar coupling. The quadrupolar term in the spin Hamiltonian can be written

$$H_{NQI} = Q_{XX}(t) \cdot I_X \cdot I_X + Q_{ZZ}(t) \cdot I_Z \cdot I_Z \quad (17)$$

where the $I_X \cdot I_X$ term leads to double quantum transitions and explains the data seen in Fig. 3(b) of the main text. This however does not directly lead to single-quantum transitions.

To drive single quantum transitions, it is necessary to have a nonzero $Q_{XZ}$ term. These can arise from misalignment of $\vec{E}_2$ such that there is some component of the RF electric field along the magnetic field or it can arise from additional internal strain fields.

If we plug the scaled values of $Q_{XX}$ into our two dimensional Rabi frequency simulation, we find an enhancement of the Rabi frequencies by a factor of 10 and reasonable agreement with data to within a factor of 4 as shown in the main text. Based on this estimate, it seems reasonable that we are driving the $^{75}$As donors through modulation of the quadrupolar interaction.

## RABI EXPERIMENTS ON THE FUNDAMENTAL TRANSITIONS

Strains perturb the donor spin system in a similar way to electric fields such that strain and electric fields can be superimposed. This has the effect of generating linear terms in the electric field response of the donor [7, 9]. For this reason, the linear response is complicated and depends on the magnitude and relative orientations of strain and electric fields in our device. We therefore focused our discussion on the subharmonic transitions which are not affected by strain to first order. However, experiments were also conducted at the fundamental frequencies for EDNMR transitions.

Two dimensional Rabi nutation experiments for both the $^{75}$As and $^{31}$P donors are shown in Fig. 7. Stark effect measurements on the same material (prior to implanting the $^{75}$As and $^{209}$Bi donors) showed a large amount of strain, presumably due to the difference in the lattice mismatch between natural and isotopically enriched silicon [8]. From those measurements, we expect an internal electric field that is randomly distributed in direction and magnitude with the average magnitude being of order 1V/$\mu$m.

For both $^{31}$P and $^{75}$As, we see a substantial improvement in the Rabi frequencies when driving the transitions at their fundamental frequencies as shown in Fig. 7. The transitions probed in this experiment are the $|m_I, m_s\rangle = |+1/2, +1/2\rangle \Longleftrightarrow |+3/2, +1/2\rangle$ for $^{75}$As and $|+1/2, +1/2\rangle \Longleftrightarrow |-1/2, +1/2\rangle$ for $^{31}$P.

To fit the experiment to data, we simply assume some proportionality constant ($\gamma_E$) between the electric field applied ($E$) and the nuclear Rabi frequency($\omega_R$) so that

$$\omega_R = \gamma_E E. \quad (18)$$

We can then quantify the Rabi frequency for the fundamental transitions in our samples and find $\gamma_E = 2\pi \cdot 270$

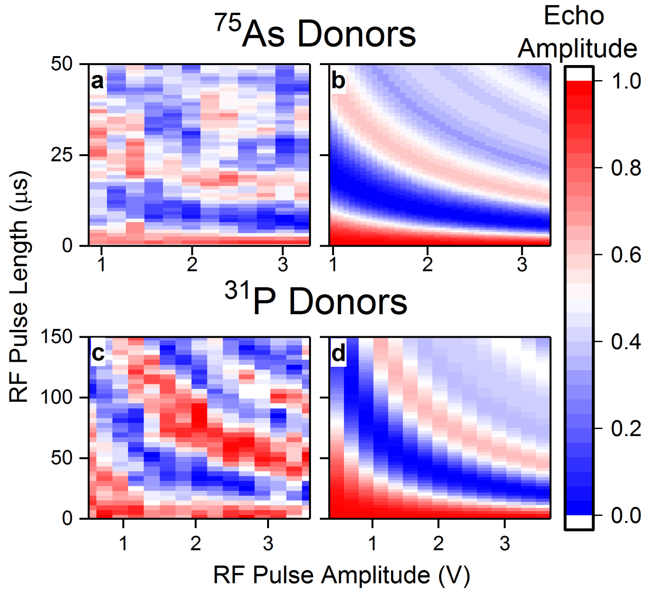


FIG. 7. Two dimensional Rabi experiment for $^{75}$As (a) and $^{31}$P (c) measured at fundamental frequencies. The simulated fits to the data are shown in (b) and (d). The $^{75}$ Data were taken at 1.9 K in a field of 250 mT.

kHz·$\mu$m/V for arsenic and $2\pi\cdot 60$ kHz·$\mu$m/V for phosphorus. Since these values are strain dependent, we should be able to enhance them by applying more strain.

---

* asigilli@princeton.edu


[1] D. M. Pozar, *Microwave engineering* (John Wiley & Sons, 2009).

[2] C. P. Wen, IEEE Transactions on Microwave Theory and Techniques **17**, 1087 (1969).

[3] A. J. Sigillito, H. Malissa, A. M. Tyryshkin, H. Riemann, N. V. Abrosimov, P. Becker, H.-J. Pohl, M. L. W. Thewalt, K. M. Itoh, J. J. L. Morton, A. A. Houck, D. I. Schuster, and S. A. Lyon, Applied Physics Letters **104**, 222407 (2014), http://dx.doi.org/10.1063/1.4881613.

[4] F. Hrubesch, G. Braunbeck, A. Voss, M. Stutzmann, and M. Brandt, Journal of Magnetic Resonance **254**, 62 (2015).

[5] A. Schweiger and G. Jeschke, *Principles of pulse electron paramagnetic resonance* (Oxford University Press on Demand, 2001).

[6] H. Malissa, D. I. Schuster, A. M. Tyryshkin, A. A. Houck, and S. A. Lyon, Review of Scientific Instruments **84**, 025116 (2013), http://dx.doi.org/10.1063/1.4792205.

[7] F. R. Bradbury, A. M. Tyryshkin, G. Sabouret, J. Bokor, T. Schenkel, and S. A. Lyon, Phys. Rev. Lett. **97**, 176404 (2006).

[8] A. J. Sigillito, A. M. Tyryshkin, and S. A. Lyon, Phys. Rev. Lett. **114**, 217601 (2015).

[9] G. Pica, G. Wolfowicz, M. Urdampilleta, M. L. W. Thewalt, H. Riemann, N. V. Abrosimov, P. Becker, H.-J. Pohl, J. J. L. Morton, R. N. Bhatt, S. A. Lyon, and B. W. Lovett, Phys. Rev. B **90**, 195204 (2014).

[10] C. C. Lo, S. Simmons, R. Lo Nardo, C. D. Weis, A. M. Tyryshkin, J. Meijer, D. Rogalla, S. A. Lyon, J. Bokor, T. Schenkel, and J. J. L. Morton, Applied Physics Letters **104**, 193502 (2014), http://dx.doi.org/10.1063/1.4876175.

[11] H. Huebl, A. R. Stegner, M. Stutzmann, M. S. Brandt, G. Vogg, F. Bensch, E. Rauls, and U. Gerstmann, Phys. Rev. Lett. **97**, 166402 (2006).

[12] D. K. Wilson and G. Feher, Phys. Rev. **124**, 1068 (1961).

[13] D. P. Franke, M. P. D. Pflüger, K. M. Itoh, and M. S. Brandt, ArXiv e-prints (2016), arXiv:1610.04138 [quant-ph].

TABLE I. Outline of the qualitative change in the photonic bandgap resonator characteristics (columns) given an increase in some lithographically defined quantities (rows).

| Increase in \ Changes the | Resonator Frequency | Resonator Q factor | Resonator Coupling | Bandgap Span | Bandgap Center Frequency | Bandgap Attenuation |
|---|---|---|---|---|---|---|
| Length of Defect ($T_C$) | ↓ | — | — | — | — | — |
| # Periods ($T_A$ and $T_B$) | — | ↑ | ↓ | — | — | ↑ |
| Length of $T_A$ and $T_B$ | ↓ | — | — | ↓ | ↓ | — |
| Impedance Step ($Z_{T_A}/Z_{T_B}$) | — | ↑ | ↓ | ↑ | — | ↑ |
